# Supplementary material for: DeepCode AI Fix: Fixing Security Vulnerabilities with Large Language Models
Source: arXiv:2402.13291 source file (2024-02-23)
Supplement: Supplementary file 1 [file appendix.tex]

\section{Some appendix}
